# Supplementary material for: Correlating Schiff moments in the light actinides with octupole moments
Source: arXiv:1807.09581 ancillary file (2018-07-25)
Supplement: Supplementary file 1 [file arxiv-supp.pdf]

# Supplemental Material for: Correlating Schiff moments in the light actinides with octupole moments

Jacek Dobaczewski,[1,2,3,4] Jonathan Engel,[5] Markus Kortelainen,[2,4] and Pierre Becker[1]

[1]*Department of Physics, University of York, Heslington, York YO10 5DD, United Kingdom*
[2]*Department of Physics, PO Box 35 (YFL), FI-40014 University of Jyväskylä, Finland*
[3]*Institute of Theoretical Physics, Faculty of Physics, University of Warsaw, ul. Pasteura 5, PL-02-093 Warsaw, Poland*
[4]*Helsinki Institute of Physics, P.O. Box 64, FI-00014 University of Helsinki, Finland*
[5]*Department of Physics and Astronomy, University of North Carolina, Chapel Hill, NC, 27516-3255, USA*

(Dated: July 25, 2018)

We show that the measured intrinsic octupole moments of $^{220}$Rn, $^{224}$Ra, and $^{226}$Ra constrain the intrinsic Schiff moments of $^{225}$Ra$^{221}$Rn, $^{223}$Rn, $^{223}$Fr, $^{225}$Ra, and $^{229}$Pa. The result is a dramatically reduced uncertainty in intrinsic Schiff moments. Direct measurements of octupole moments in odd nuclei will reduce the uncertainty even more. The only significant source of nuclear-physics error in the laboratory Schiff moments will then be the intrinsic matrix elements of the time-reversal non-invariant interaction produced by CP-violating fundamental physics. Those matrix elements are also correlated with octupole moments, but with a larger systematic uncertainty.

Figure 4 compares (laboratory) reduced matrix elements of the Schiff and octupole operators with their values in the rigid-deformation approximation, for increasingly large numbers of oscillator shells in the single-particle space underlying our calculations. The intrinsic state $|\Phi_0\rangle$ for panels (a) and (b), for $^{225}$Ra is oriented so that $S_0 > 0$ and $K = +\frac{1}{2}$, leading to $\langle\frac{1}{2}^+||\hat{S}_0||\frac{1}{2}^-\rangle_{\rm rigid} = +2S_0/\sqrt{6}$, where phases of the parity-projected states are fixed by the relation $|J^\pm\rangle = (|\Phi_0\rangle \pm \hat{P}\,|\Phi_0\rangle)/\sqrt{2}$. As it turns out, in the actinides the overlaps and matrix elements between the parity-reversed intrinsic states are very small and can safely be neglected.

Panels (a) and (b) of the figure show that for the Schiff operator the rigid-deformation approximation turns out to be very good; it induces an error of only about 1.5%. These panels also show the error from extrapolating our results to a single-particle space with an infinite number of harmonic-oscillator shells to be even smaller, only about 0.02%. For calculations with 20 oscillator shells, which lead to a reasonable balance between CPU time and precision, the two errors have similar magnitude and opposite sign. We thus use this basis for all calculations performed with Skyrme functionals.

Figures 4(c) and (d) show that the rigid-deformation approximation for the octupole operator $\hat{Q}^3$ is in $^{224}$Ra is even better. To obtain these results, we orient the intrinsic state so that $Q_0^3 > 0$ and $K = 0$, leading to $\langle 0^+||\hat{Q}_0^3||3^-\rangle_{\rm rigid} = -Q_0^3$. Again we see that the extrapolation to infinite number of shells gives a very small error of about 0.01% and that using 20 HO shells allows for better than 1% precision. The accuracy of all these approximations means that we can consider the Schiff and octupole transition matrix elements to be directly proportional to the corresponding intrinsic moments.

In Tables II and III, we show results of calculations for the intrinsic Schiff ($S_0$) and octupole ($Q_0^3$) moments determined in this work. These data are the baseline of

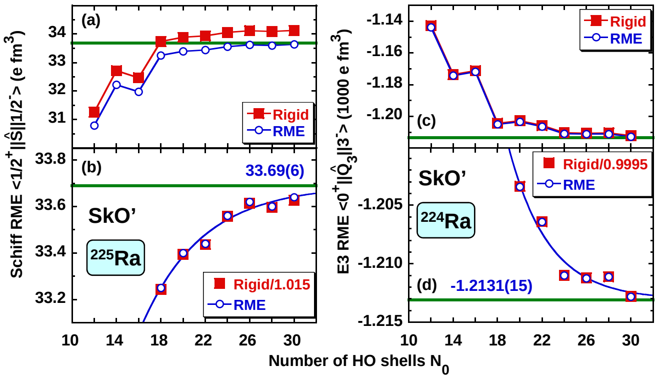


FIG. 4. (Color online) Reduced matrix element of the Schiff operator $\hat{S}$ between the ground state and its parity-doublet partner in $^{225}$Ra (left), and of the octupole operator $\hat{Q}^3$ between the $0^+$ ground state and the $3^-$ member of the $K = 0$ rotational band (right), as functions of the number of harmonic-oscillator shells in which the calculations is done. The full result is represented by open blue circles and the rigid-deformation approximation (6) by red squares. Panels (a) and (c) are the reduced matrix elements themselves. Panels (b) and (d) are the reduced matrix elements and the rigid-rotor approximations each divided by 1.015 (c) or 0.9995 (d), and magnified in extended scale. Horizontal lines at 33.69(6) e fm$^3$ and $-1.2131(15)$ e fm$^3$ are the results of exponential extrapolation to an infinite number of shells. All results were obtained with the Skyrme functional SkO′.

the regression analysis that correlates the intrinsic Schiff and octupole moments in $^{221}$Rn, $^{223}$Rn, $^{223}$Fr, $^{225}$Ra, and $^{229}$Pa with the intrinsic octupole moments in $^{224}$Ra, $^{226}$Ra and $^{220}$Rn. In each case, the linear-regression coefficients $a$ and $b$,

$$S_0 = a + bQ_0^3, \tag{10}$$

are determined by a minimization of the penalty function

TABLE II. Intrinsic Schiff moments $S_0$ (in e fm$^3$) of $^{221}$Rn, $^{223}$Rn, $^{223}$Fr, $^{225}$Ra, and $^{229}$Pa determined in this work for functionals SIII [2], SkM* [3], SkO′ [4], SkX$_c$ [5], SLy4 [6], and UNEDF0 [7] (within the BCS method), and D1S [8] and UNEDF0 [7] (within the HFB method).

| EDF | method | $^{221}$Rn | $^{223}$Rn | $^{223}$Fr | $^{225}$Ra | $^{229}$Pa |
|---|---|---|---|---|---|---|
| SIII | BCS | 13.9 | 6.9 | 24.0 | 27.0 | 37.6 |
| SkM* | BCS | 21.6 | 30.7 | 32.5 | 38.9 | 46.4 |
| SkO′ | BCS | 11.4 | 18.3 | 23.2 | 31.5 | 40.9 |
| SkX$_c$ | BCS | 6.4 | 13.8 | 18.3 | 23.6 | 34.6 |
| SLy4 | BCS | 20.4 | 26.2 | 28.8 | 36.8 | 46.0 |
| UNEDF0 | BCS | 10.6 | 17.2 | 19.9 | 27.9 | 33.4 |
| D1S | HFB | 27.6 | 30.9 | 34.3 | 43.4 | 52.0 |
| UNEDF0 | HFB | 20.5 | 23.5 | 25.1 | 32.7 | 32.9 |

$\chi^2$ [1],

$$\chi^2 = \sum_i \left(S_0(i) - a - bQ_0^3(i)\right)^2, \tag{11}$$

where $S_0(i)$ and $Q_0^3(i)$ are, respectively, the intrinsic Schiff and octupole moments calculated for one of $N_d = 8$ functionals, $i = 1 \ldots N_d$, considered in this work; see Tables II and III. Tables IV–IX list regression coefficients $a$ and $b$ obtained for all cases considered in this work.

Since we do not have error estimates for the calculated moments, we do not weigh different terms of the penalty function differently. Instead, we employ a penalty function normalized by the Birge factor $s$ [1, 9],

$$\chi^2_{\text{norm}} = \frac{\chi^2}{s} \qquad \text{for} \qquad s = \frac{\chi_0^2}{N_d - N_p}, \tag{12}$$

where $\chi_0^2$ is the value of the penalty function at the minimum and $N_p = 2$ is the number of parameters. With such a choice, the covariance matrix of the fit can be determined as

$$\mathcal{C} = s\mathcal{M}, \tag{13}$$

where $\mathcal{M}$ is the Hessian matrix [1] calculated at the minimum of the penalty function. Tables IV–IX list elements $\mathcal{C}_{aa}$, $\mathcal{C}_{ab}$, and $\mathcal{C}_{bb}$ of the covariance matrices obtained for all cases considered in this work.

Inserting experimental octupole moments $Q_0^3(\text{exp})$ into Eq. (10), we obtain estimates of the intrinsic Schiff moments,

$$S_0(\text{est}) = a + bQ_0^3(\text{exp}). \tag{14}$$

Derivatives of the estimates with respect to the regression coefficients read

$$\frac{\partial S_0(\text{est})}{\partial a} = 1, \qquad \frac{\partial S_0(\text{est})}{\partial b} = Q_0^3(\text{exp}), \tag{15}$$

and thus we obtain estimates [1] of theoretical uncertainties $\Delta S_0(\text{the})$ in the Schiff moments $S_0(\text{est})$ as,

$$\Delta S_0(\text{the})^2 = \mathcal{C}_{aa} + 2\mathcal{C}_{ab}Q_0^3(\text{exp}) + \mathcal{C}_{bb}Q_0^3(\text{exp})^2. \tag{16}$$

The experimental uncertainties $\Delta Q_0^3(\text{exp})$ in the $Q_0^3(\text{exp})$ induce, through Eq. (14), experimental uncertainties $\Delta S_0(\text{exp})$ in the Schiff moments $S_0(\text{est})$, that is,

$$\Delta S_0(\text{exp}) = b\Delta Q_0^3(\text{exp}). \tag{17}$$

Finally, total uncertainties $\Delta S_0(\text{est})$ estimated in this work are calculated as

$$\Delta S_0(\text{est}) = \sqrt{\Delta S_0(\text{the})^2 + \Delta S_0(\text{exp})^2}. \tag{18}$$

Tables X and XI list values of the estimated intrinsic Schiff and octupole moments obtained for all cases considered in this work. Their estimated total uncertainties are also given.

Figures 5–19 and 20–34 show correlations between intrinsic Schiff/octupole moments and octupole moments of $^{224}$Ra, $^{226}$Ra, and $^{220}$Rn. Circles and diamonds correspond to results obtained within the BCS and HFB methods, respectively; see Tables II and III. Lines show the linear approximations (10) for the regression coefficients $a$ and $b$ listed in Tables IV–IX. Triangles with error bars indicate the propagated values of intrinsic Schiff and octupole moments (14) and their total uncertainties (18). The experimental octupole moments used in our analysis are $Q_0^3(\text{exp}) = 940(30)$ e fm$^3$ for $^{224}$Ra [10], $Q_0^3(\text{exp}) = 1080(30)$ e fm$^3$ for $^{226}$Ra [11], and $Q_0^3(\text{exp}) = 810(50)$ e fm$^3$ for $^{220}$Rn [10].

In Tables XII–XVI, we show for $^{221}$Rn, $^{223}$Rn, $^{223}$Fr, $^{225}$Ra, and $^{229}$Pa the calculated average values of the five different terms in the $\hat{V}_{PT}$ interaction (4), so that

$$\langle \hat{V}_{PT} \rangle = v_0\, g\, \bar{g}_0 + v_1\, g\, \bar{g}_1 + v_2\, g\, \bar{g}_2 + w_1\, \bar{c}_1 + w_2\, \bar{c}_2. \tag{19}$$

Then, Tables XVII–XXXI show regression coefficients $a$ and $b$ from Eq. (10) and elements of the covariance matrices from Eq. (13), corresponding to the coefficients $a_0$, $a_1$, and $a_2$ (in e fm$^3$), and $b_1$ and $b_2$ (in 0.1 e fm$^3$) (see Eq. (5)), determined for $^{221}$Rn, $^{223}$Rn, $^{223}$Fr, $^{225}$Ra, and $^{229}$Pa, and correlated with the intrinsic octupole moments $Q_0^3$ (in 1000 e fm$^3$) of $^{224}$Ra, $^{226}$Ra, and $^{220}$Rn. Each of the coefficients is related to the corresponding intrinsic Schiff moment $S_0$ and average value (19) as

$$a_i = -\frac{2J}{J+1}\frac{S_0 v_i}{\Delta E} \quad \text{and} \quad b_i = -\frac{2J}{J+1}\frac{S_0 w_i}{\Delta E}. \tag{20}$$

Figures 35–49 and 50–64 show the corresponding correlations of coefficients $a_i$ and $b_i$ with intrinsic octupole moments. Finally, Table XXXII shows coefficients $a_0$, $a_1$, $a_2$, $b_1$, and $b_2$ (in e fm$^3$), determined for $^{221}$Rn, $^{223}$Rn, $^{223}$Fr, $^{225}$Ra, and $^{229}$Pa from the experimental octupole moments of $^{224}$Ra, $^{226}$Ra, and $^{220}$Rn.

TABLE III. Same as in Table II but for the intrinsic octupole moments $Q_0^3$ (in 1000 $\mathrm{e\,fm}^3$), and with results for $^{224}$Ra, $^{226}$Ra and $^{220}$Rn.

| EDF | method | $^{221}$Rn | $^{223}$Rn | $^{223}$Fr | $^{225}$Ra | $^{229}$Pa | $^{224}$Ra | $^{226}$Ra | $^{220}$Rn |
|---|---|---|---|---|---|---|---|---|---|
| SIII | BCS | 0.7041 | 0.3032 | 0.9407 | 0.9515 | 1.2378 | 1.0070 | 0.9396 | 0.5705 |
| SkM* | BCS | 1.1898 | 1.2682 | 1.2079 | 1.3006 | 1.4098 | 1.3717 | 1.2900 | 1.1070 |
| SkO′ | BCS | 0.5405 | 0.7824 | 0.8689 | 1.0753 | 1.3158 | 0.9970 | 1.0993 | 0.4298 |
| SkX$_c$ | BCS | 0.3618 | 0.6461 | 0.7409 | 0.8593 | 1.1719 | 0.8757 | 0.8918 | 0.1406 |
| SLy4 | BCS | 0.8625 | 1.0448 | 1.0263 | 1.2130 | 1.4275 | 1.1674 | 1.2127 | 0.7209 |
| UNEDF0 | BCS | 0.7521 | 0.8781 | 0.8743 | 1.0753 | 1.1036 | 1.0288 | 1.0468 | 0.6671 |
| D1S | HFB | 1.0590 | 1.1319 | 1.1176 | 1.3253 | 1.5118 | 1.2736 | 1.2403 | 0.8765 |
| UNEDF0 | HFB | 0.9014 | 1.0279 | 0.9883 | 1.1926 | 1.0138 | 1.1183 | 1.1177 | 0.9019 |

TABLE IV. Regression coefficients $a$ and $b$, Eq. (10), and elements of the covariance matrices, Eq. (13), corresponding to the intrinsic Schiff moments $S_0$ (in $e\,\mathrm{fm}^3$) correlated with the $^{224}$Ra intrinsic octupole moments $Q_0^3$ (in 1000 $e\,\mathrm{fm}^3$), determined for $^{221}$Rn, $^{223}$Rn, $^{223}$Fr, $^{225}$Ra, and $^{229}$Pa. See also Figs. 5–9.

| | $^{221}$Rn | $^{223}$Rn | $^{223}$Fr | $^{225}$Ra | $^{229}$Pa |
|---|---|---|---|---|---|
| $a$ | −26.2500 | −28.6654 | −10.5570 | −8.5960 | 4.9692 |
| $b$ | 38.7352 | 44.8921 | 32.8702 | 37.3967 | 32.1338 |
| $\mathcal{C}_{aa}$ | 84.8368 | 145.2036 | 33.5428 | 60.1704 | 180.5238 |
| $\mathcal{C}_{ab}$ | −75.3655 | −128.9929 | −29.7981 | −53.4529 | −160.3699 |
| $\mathcal{C}_{bb}$ | 68.2079 | 116.7422 | 26.9681 | 48.3764 | 145.1393 |

TABLE V. Same as in Table IV but for the correlation with the $^{226}$Ra intrinsic octupole moments. See also Figs. 10–14.

| | $^{221}$Rn | $^{223}$Rn | $^{223}$Fr | $^{225}$Ra | $^{229}$Pa |
|---|---|---|---|---|---|
| $a$ | −29.6156 | −40.6164 | −13.2217 | −16.0615 | −1.1280 |
| $b$ | 41.7874 | 55.7162 | 35.2870 | 44.1597 | 37.6574 |
| $\mathcal{C}_{aa}$ | 153.6314 | 90.3317 | 77.3931 | 52.1082 | 219.6531 |
| $\mathcal{C}_{ab}$ | −137.0883 | −80.6048 | −69.0594 | −46.4972 | −196.0008 |
| $\mathcal{C}_{bb}$ | 124.0871 | 72.9604 | 62.5099 | 42.0874 | 177.4124 |

TABLE VI. Same as in Table IV but for the correlation with the $^{220}$Rn intrinsic octupole moments. See also Figs. 15–19.

| | $^{221}$Rn | $^{223}$Rn | $^{223}$Fr | $^{225}$Ra | $^{229}$Pa |
|---|---|---|---|---|---|
| $a$ | 3.2877 | 7.1303 | 15.7120 | 21.2451 | 33.2468 |
| $b$ | 19.5959 | 20.4010 | 14.8503 | 16.9623 | 10.6802 |
| $\mathcal{C}_{aa}$ | 14.7907 | 32.6748 | 12.2442 | 17.7279 | 38.8214 |
| $\mathcal{C}_{ab}$ | −18.6158 | −41.1248 | −15.4107 | −22.3125 | −48.8610 |
| $\mathcal{C}_{bb}$ | 27.5061 | 60.7647 | 22.7704 | 32.9682 | 72.1955 |

TABLE VII. Same as in Table IV but for the intrinsic octupole moments. See also Figs. 20–24.

| | $^{221}$Rn | $^{223}$Rn | $^{223}$Fr | $^{225}$Ra | $^{229}$Pa |
|---|---|---|---|---|---|
| $a$ | −0.9786 | −0.7973 | −0.0284 | 0.0747 | 0.5635 |
| $b$ | 1.6064 | 1.5228 | 0.9041 | 0.9498 | 0.6431 |
| $100 \times \mathcal{C}_{aa}$ | 3.5038 | 26.5655 | 0.5420 | 2.6656 | 15.0416 |
| $100 \times \mathcal{C}_{ab}$ | −3.1126 | −23.5997 | −0.4815 | −2.3680 | −13.3623 |
| $100 \times \mathcal{C}_{bb}$ | 2.8170 | 21.3584 | 0.4357 | 2.1431 | 12.0933 |

TABLE VIII. Same as in Table V but for the intrinsic octupole moments. See also Figs. 25–29.

| | $^{221}$Rn | $^{223}$Rn | $^{223}$Fr | $^{225}$Ra | $^{229}$Pa |
|---|---|---|---|---|---|
| $a$ | −1.0018 | −1.2490 | −0.0523 | −0.1215 | 0.4252 |
| $b$ | 1.6277 | 1.9319 | 0.9259 | 1.1275 | 0.7683 |
| $100 \times \mathcal{C}_{aa}$ | 19.3367 | 19.8888 | 5.0118 | 1.5062 | 18.4779 |
| $100 \times \mathcal{C}_{ab}$ | −17.2546 | −17.7472 | −4.4721 | −1.3440 | −16.4882 |
| $100 \times \mathcal{C}_{bb}$ | 15.6182 | 16.0641 | 4.0480 | 1.2166 | 14.9245 |

TABLE IX. Same as in Table VI but for the intrinsic octupole moments. See also Figs. 30–34.

| | $^{221}$Rn | $^{223}$Rn | $^{223}$Fr | $^{225}$Ra | $^{229}$Pa |
|---|---|---|---|---|---|
| $a$ | 0.2075 | 0.3877 | 0.6624 | 0.7968 | 1.1636 |
| $b$ | 0.8702 | 0.7353 | 0.4554 | 0.4836 | 0.1632 |
| $100 \times \mathcal{C}_{aa}$ | 0.2990 | 4.4320 | 0.3153 | 0.5594 | 2.6964 |
| $100 \times \mathcal{C}_{ab}$ | −0.3763 | −5.5782 | −0.3968 | −0.7041 | −3.3937 |
| $100 \times \mathcal{C}_{bb}$ | 0.5560 | 8.2422 | 0.5864 | 1.0403 | 5.0145 |

TABLE X. Intrinsic Schiff moments $S_0$(est) (in $e\,\mathrm{fm}^3$), Eq. (14), of $^{221}$Rn, $^{223}$Rn, $^{223}$Fr, $^{225}$Ra, and $^{229}$Pa, and their uncertainties, Eq. (18), estimated in this work from the experimental octupole moments of $^{224}$Ra [10], $^{226}$Ra [11], and $^{220}$Rn [10]. See also Fig. 4(b) of the Letter.

| | $K$ | from $^{224}$Ra | from $^{226}$Ra | from $^{220}$Rn |
|---|---|---|---|---|
| $^{221}$Rn | $\frac{7}{2}$ | 10.2(2.2) | 15.5(2.0) | 19.2(1.9) |
| $^{223}$Rn | $\frac{7}{2}$ | 13.5(2.8) | 19.6(2.0) | 23.7(2.6) |
| $^{223}$Fr | $\frac{3}{2}$ | 20.3(1.5) | 24.9(1.5) | 27.7(1.7) |
| $^{225}$Ra | $\frac{1}{2}$ | 26.6(1.9) | 31.6(1.6) | 35.0(2.0) |
| $^{229}$Pa | $\frac{5}{2}$ | 35.2(2.9) | 39.5(2.1) | 41.9(2.7) |

TABLE XI. Same as in Table X but for the intrinsic octupole moments $Q_0^3$ (in 1000 $e\,\mathrm{fm}^3$). See also Fig. 4(a) of the Letter.

| | $K$ | from $^{224}$Ra | from $^{226}$Ra | from $^{220}$Rn |
|---|---|---|---|---|
| $^{221}$Rn | $\frac{7}{2}$ | 0.53(6) | 0.76(7) | 0.91(5) |
| $^{223}$Rn | $\frac{7}{2}$ | 0.63(11) | 0.84(8) | 0.98(10) |
| $^{223}$Fr | $\frac{3}{2}$ | 0.82(3) | 0.95(4) | 1.03(3) |
| $^{225}$Ra | $\frac{1}{2}$ | 0.97(4) | 1.10(4) | 1.19(4) |
| $^{229}$Pa | $\frac{5}{2}$ | 1.17(8) | 1.25(6) | 1.30(7) |

TABLE XII. Coefficients $v_0$, $v_1$, $v_2$, $w_1$, and $w_2$ (in keV), Eq. (19), determined in $^{221}$Rn for functionals SIII [2], SkM* [3], SkO′ [4], SkX$_c$ [5], SLy4 [6], and UNEDF0 [7] within the BCS method.

| EDF | $v_0$ | $v_1$ | $v_2$ | $w_1$ | $w_2$ |
|---|---|---|---|---|---|
| SIII | 2.979 | 9.876 | −3.835 | 0.768 | 0.028 |
| SkM* | −0.986 | 9.183 | −3.847 | 0.154 | 0.103 |
| SkO′ | 1.148 | 2.471 | −0.940 | 0.260 | 0.465 |
| SkX$_c$ | 2.915 | 3.257 | −1.021 | 0.483 | 0.322 |
| SLy4 | 0.720 | 6.904 | −2.203 | 0.290 | 0.042 |
| UNEDF0 | 0.088 | 3.709 | −1.720 | 0.117 | 0.193 |

TABLE XIII. Same as in Table XII but for $^{223}$Rn.

| EDF | $v_0$ | $v_1$ | $v_2$ | $w_1$ | $w_2$ |
|---|---|---|---|---|---|
| SIII | 2.742 | 13.342 | −4.701 | 1.224 | 0.012 |
| SkM* | −0.627 | 11.372 | −4.432 | 0.350 | 0.184 |
| SkO′ | 1.224 | 4.633 | −2.051 | 0.478 | 0.723 |
| SkX$_c$ | 3.630 | 7.471 | −2.846 | 0.868 | 0.416 |
| SLy4 | 0.758 | 12.568 | −3.559 | 0.782 | −0.096 |
| UNEDF0 | 0.247 | 5.638 | −2.490 | 0.209 | 0.237 |

TABLE XIV. Same as in Table XII but for $^{223}$Fr.

| EDF | $v_0$ | $v_1$ | $v_2$ | $w_1$ | $w_2$ |
|---|---|---|---|---|---|
| SIII | −4.697 | 13.877 | −2.972 | −0.399 | 0.534 |
| SkM* | 1.701 | −6.495 | 8.161 | −1.002 | 1.166 |
| SkO′ | −0.730 | 8.595 | −1.787 | −0.362 | 0.482 |
| SkX$_c$ | −2.743 | 13.578 | −4.207 | −0.246 | 0.065 |
| SLy4 | 1.898 | 5.022 | 0.733 | −0.888 | 0.198 |
| UNEDF0 | 4.218 | −10.729 | 5.733 | −0.570 | 0.736 |

TABLE XV. Same as in Table XII but for $^{225}$Ra.

| EDF | $v_0$ | $v_1$ | $v_2$ | $w_1$ | $w_2$ |
|---|---|---|---|---|---|
| SIII | 0.346 | 12.398 | −7.216 | 0.462 | −0.887 |
| SkM* | −6.432 | 37.628 | −21.121 | −0.932 | −0.641 |
| SkO′ | −0.647 | 6.505 | −5.928 | 0.361 | 0.455 |
| SkX$_c$ | 1.532 | 9.025 | −5.624 | 0.506 | −0.243 |
| SLy4 | −1.733 | 27.266 | −15.562 | −0.379 | −0.515 |
| UNEDF0 | −2.184 | 22.951 | −11.687 | −0.049 | −0.586 |

TABLE XVI. Same as in Table XII but for $^{229}$Pa.

| EDF | $v_0$ | $v_1$ | $v_2$ | $w_1$ | $w_2$ |
|---|---|---|---|---|---|
| SIII | 4.027 | 2.220 | −2.108 | −0.500 | −0.711 |
| SkM* | 6.769 | −15.055 | 9.218 | −1.104 | 0.527 |
| SkO′ | 4.077 | −0.045 | 0.028 | −0.935 | −1.067 |
| SkX$_c$ | 6.471 | 0.123 | −0.915 | −0.687 | −0.894 |
| SLy4 | 9.061 | −11.310 | 3.855 | −0.706 | −0.795 |
| UNEDF0 | 8.511 | −15.224 | 6.640 | −0.856 | −0.008 |

TABLE XVII. Regression coefficients $a$ and $b$, Eq. (10), and elements of the covariance matrices, Eq. (13), corresponding to the coefficients $a_0$, $a_1$, and $a_2$ (in e fm$^3$), and $b_1$ and $b_2$ (in 0.1 e fm$^3$), Eq. (5), determined for $^{221}$Rn and correlated with the $^{224}$Ra intrinsic octupole moments $Q^3_0$ (in 1000 e fm$^3$). See also Figs. 35 and 50.

| | $a_0$ | $a_1$ | $a_2$ | $b_1$ | $b_2$ |
|---|---|---|---|---|---|
| $a$ | -1.7024 | 2.9971 | -1.2925 | -0.3645 | -0.2835 |
| $b$ | 1.4033 | -3.9725 | 1.6572 | 0.1831 | 0.1760 |
| $\mathcal{C}_{aa}$ | 0.2730 | 1.9239 | 0.2921 | 0.0902 | 0.0613 |
| $\mathcal{C}_{ab}$ | -0.2487 | -1.7526 | -0.2661 | -0.0822 | -0.0559 |
| $\mathcal{C}_{bb}$ | 0.2315 | 1.6309 | 0.2476 | 0.0764 | 0.0520 |

TABLE XVIII. Same as in Table XVII, for $^{223}$Rn correlated with $^{224}$Ra. See also Figs. 36 and 51.

| | $a_0$ | $a_1$ | $a_2$ | $b_1$ | $b_2$ |
|---|---|---|---|---|---|
| $a$ | -1.6867 | 2.8707 | -0.9661 | -0.4360 | -0.3826 |
| $b$ | 1.3545 | -4.4855 | 1.5559 | 0.1030 | 0.2443 |
| $\mathcal{C}_{aa}$ | 0.2152 | 4.0690 | 0.2384 | 0.2766 | 0.2089 |
| $\mathcal{C}_{ab}$ | -0.1960 | -3.7068 | -0.2171 | -0.2520 | -0.1903 |
| $\mathcal{C}_{bb}$ | 0.1824 | 3.4494 | 0.2021 | 0.2345 | 0.1771 |

TABLE XIX. Same as in Table XVII, for $^{223}$Fr correlated with $^{224}$Ra. See also Figs. 37 and 52.

| | $a_0$ | $a_1$ | $a_2$ | $b_1$ | $b_2$ |
|---|---|---|---|---|---|
| $a$ | 1.5668 | -6.1099 | 4.1377 | -0.7848 | 0.7818 |
| $b$ | -1.4874 | 5.2258 | -4.0615 | 0.9540 | -0.9299 |
| $\mathcal{C}_{aa}$ | 1.4547 | 13.5818 | 1.9056 | 0.0181 | 0.1208 |
| $\mathcal{C}_{ab}$ | -1.3252 | -12.3727 | -1.7359 | -0.0165 | -0.1101 |
| $\mathcal{C}_{bb}$ | 1.2332 | 11.5137 | 1.6154 | 0.0154 | 0.1024 |

TABLE XX. Same as in Table XVII, for $^{225}$Ra correlated with $^{224}$Ra. See also Figs. 38 and 53.

| | $a_0$ | $a_1$ | $a_2$ | $b_1$ | $b_2$ |
|---|---|---|---|---|---|
| $a$ | -6.7993 | 29.8202 | -16.0493 | -3.5057 | -1.1473 |
| $b$ | 6.9963 | -35.0625 | 19.1687 | 3.3411 | 1.4245 |
| $\mathcal{C}_{aa}$ | 1.4992 | 29.3508 | 5.1372 | 0.2915 | 1.4433 |
| $\mathcal{C}_{ab}$ | -1.3657 | -26.7377 | -4.6799 | -0.2656 | -1.3148 |
| $\mathcal{C}_{bb}$ | 1.2709 | 24.8816 | 4.3550 | 0.2471 | 1.2236 |

TABLE XXI. Same as in Table XVII, for $^{229}$Pa correlated with $^{224}$Ra. See also Figs. 39 and 54.

| | $a_0$ | $a_1$ | $a_2$ | $b_1$ | $b_2$ |
|---|---|---|---|---|---|
| $a$ | 1.1849 | -8.2439 | 5.2133 | -0.5423 | 1.6333 |
| $b$ | -2.3711 | 9.0912 | -5.4869 | 0.8996 | -1.3073 |
| $\mathcal{C}_{aa}$ | 1.7892 | 10.6864 | 2.5689 | 0.0915 | 0.6588 |
| $\mathcal{C}_{ab}$ | -1.6299 | -9.7350 | -2.3402 | -0.0834 | -0.6001 |
| $\mathcal{C}_{bb}$ | 1.5167 | 9.0592 | 2.1777 | 0.0776 | 0.5585 |

TABLE XXII. Same as in Table XVII, for $^{221}$Rn correlated with $^{226}$Ra. See also Figs. 40 and 55.

| | $a_0$ | $a_1$ | $a_2$ | $b_1$ | $b_2$ |
|---|---|---|---|---|---|
| $a$ | -1.9276 | 2.2027 | -0.9132 | -0.5189 | -0.1496 |
| $b$ | 1.6047 | -3.2169 | 1.2976 | 0.3251 | 0.0511 |
| $\mathcal{C}_{aa}$ | 0.3185 | 5.2681 | 0.8974 | 0.0955 | 0.0885 |
| $\mathcal{C}_{ab}$ | -0.2900 | -4.7967 | -0.8171 | -0.0869 | -0.0806 |
| $\mathcal{C}_{bb}$ | 0.2685 | 4.4412 | 0.7565 | 0.0805 | 0.0746 |

TABLE XXIII. Same as in Table XVIII, for $^{223}$Rn correlated with $^{226}$Ra. See also Figs. 41 and 56.

| | $a_0$ | $a_1$ | $a_2$ | $b_1$ | $b_2$ |
|---|---|---|---|---|---|
| $a$ | -1.9141 | 2.3542 | -0.7007 | -0.5777 | -0.2116 |
| $b$ | 1.5582 | -3.9846 | 1.3023 | 0.2338 | 0.0847 |
| $\mathcal{C}_{aa}$ | 0.2384 | 7.9694 | 0.7040 | 0.3383 | 0.2849 |
| $\mathcal{C}_{ab}$ | -0.2171 | -7.2562 | -0.6410 | -0.3081 | -0.2594 |
| $\mathcal{C}_{bb}$ | 0.2010 | 6.7185 | 0.5935 | 0.2852 | 0.2402 |

TABLE XXIV. Same as in Table XIX, for $^{223}$Fr correlated with $^{226}$Ra. See also Figs. 42 and 57.

| | $a_0$ | $a_1$ | $a_2$ | $b_1$ | $b_2$ |
|---|---|---|---|---|---|
| $a$ | 2.2012 | -6.3080 | 4.1191 | -0.8744 | 0.6984 |
| $b$ | -2.0673 | 5.3830 | -4.0238 | 1.0322 | -0.8479 |
| $\mathcal{C}_{aa}$ | 1.4033 | 18.8294 | 3.7798 | 0.0472 | 0.2631 |
| $\mathcal{C}_{ab}$ | -1.2777 | -17.1443 | -3.4415 | -0.0430 | -0.2396 |
| $\mathcal{C}_{bb}$ | 1.1830 | 15.8738 | 3.1865 | 0.0398 | 0.2218 |

TABLE XXV. Same as in Table XX, for $^{225}$Ra correlated with $^{226}$Ra. See also Figs. 43 and 58.

| | $a_0$ | $a_1$ | $a_2$ | $b_1$ | $b_2$ |
|---|---|---|---|---|---|
| $a$ | -6.9329 | 30.3626 | -16.9315 | -3.6325 | -0.3501 |
| $b$ | 7.0848 | -35.3883 | 19.8892 | 3.4417 | 0.6792 |
| $\mathcal{C}_{aa}$ | 5.3113 | 125.3457 | 26.5461 | 1.0293 | 2.4511 |
| $\mathcal{C}_{ab}$ | -4.8360 | -114.1280 | -24.1704 | -0.9372 | -2.2317 |
| $\mathcal{C}_{bb}$ | 4.4776 | 105.6708 | 22.3793 | 0.8677 | 2.0664 |

TABLE XXVI. Same as in Table XXI, for $^{229}$Pa correlated with $^{226}$Ra. See also Figs. 44 and 59.

| | $a_0$ | $a_1$ | $a_2$ | $b_1$ | $b_2$ |
|---|---|---|---|---|---|
| $a$ | 1.7846 | -9.2466 | 5.5517 | -0.7259 | 1.2338 |
| $b$ | -2.9145 | 9.9738 | -5.7726 | 1.0651 | -0.9308 |
| $\mathcal{C}_{aa}$ | 1.8504 | 14.9382 | 4.6272 | 0.0821 | 1.2169 |
| $\mathcal{C}_{ab}$ | -1.6848 | -13.6013 | -4.2131 | -0.0748 | -1.1080 |
| $\mathcal{C}_{bb}$ | 1.5599 | 12.5934 | 3.9009 | 0.0692 | 1.0259 |

TABLE XXVII. Same as in Table XVII, for $^{221}$Rn correlated with $^{220}$Rn. See also Figs. 45 and 60.

| | $a_0$ | $a_1$ | $a_2$ | $b_1$ | $b_2$ |
|---|---|---|---|---|---|
| $a$ | -0.6478 | -0.0155 | -0.0533 | -0.2263 | -0.1646 |
| $b$ | 0.7482 | -2.0729 | 0.8938 | 0.0965 | 0.1157 |
| $\mathcal{C}_{aa}$ | 0.0312 | 0.2424 | 0.0317 | 0.0100 | 0.0063 |
| $\mathcal{C}_{ab}$ | -0.0417 | -0.3240 | -0.0423 | -0.0134 | -0.0084 |
| $\mathcal{C}_{bb}$ | 0.0689 | 0.5347 | 0.0698 | 0.0221 | 0.0139 |

TABLE XXVIII. Same as in Table XVIII, for $^{223}$Rn correlated with $^{220}$Rn. See also Figs. 46 and 61.

| | $a_0$ | $a_1$ | $a_2$ | $b_1$ | $b_2$ |
|---|---|---|---|---|---|
| $a$ | -0.6879 | -0.6207 | 0.2295 | -0.3784 | -0.2164 |
| $b$ | 0.7538 | -2.1926 | 0.7860 | 0.0876 | 0.1590 |
| $\mathcal{C}_{aa}$ | 0.0195 | 0.5643 | 0.0356 | 0.0301 | 0.0223 |
| $\mathcal{C}_{ab}$ | -0.0260 | -0.7543 | -0.0476 | -0.0403 | -0.0297 |
| $\mathcal{C}_{bb}$ | 0.0429 | 1.2448 | 0.0785 | 0.0665 | 0.0491 |

TABLE XXIX. Same as in Table XIX, for $^{223}$Fr correlated with $^{220}$Rn. See also Figs. 47 and 62.

| | $a_0$ | $a_1$ | $a_2$ | $b_1$ | $b_2$ |
|---|---|---|---|---|---|
| $a$ | 0.4801 | -2.4586 | 1.1437 | -0.0463 | 0.0964 |
| $b$ | -0.8443 | 3.2417 | -2.2616 | 0.4731 | -0.5177 |
| $\mathcal{C}_{aa}$ | 0.1529 | 1.2082 | 0.1711 | 0.0064 | 0.0113 |
| $\mathcal{C}_{ab}$ | -0.2043 | -1.6150 | -0.2287 | -0.0086 | -0.0151 |
| $\mathcal{C}_{bb}$ | 0.3372 | 2.6651 | 0.3774 | 0.0141 | 0.0249 |

TABLE XXX. Same as in Table XX, for $^{225}$Ra correlated with $^{220}$Rn. See also Figs. 48 and 63.

| | $a_0$ | $a_1$ | $a_2$ | $b_1$ | $b_2$ |
|---|---|---|---|---|---|
| $a$ | -1.4672 | 2.9678 | -1.2435 | -0.9254 | -0.1505 |
| $b$ | 3.6075 | -17.8648 | 9.5596 | 1.6668 | 0.8813 |
| $\mathcal{C}_{aa}$ | 0.2920 | 7.2873 | 2.2285 | 0.0825 | 0.1384 |
| $\mathcal{C}_{ab}$ | -0.3903 | -9.7406 | -2.9788 | -0.1103 | -0.1850 |
| $\mathcal{C}_{bb}$ | 0.6441 | 16.0740 | 4.9157 | 0.1820 | 0.3053 |

TABLE XXXI. Same as in Table XXI, for $^{229}$Pa correlated with $^{220}$Rn. See also Figs. 49 and 64.

| | $a_0$ | $a_1$ | $a_2$ | $b_1$ | $b_2$ |
|---|---|---|---|---|---|
| $a$ | -0.6553 | -1.4354 | 1.0717 | 0.1638 | 0.6913 |
| $b$ | -1.1680 | 4.8861 | -2.8957 | 0.4301 | -0.7637 |
| $\mathcal{C}_{aa}$ | 0.2277 | 1.1822 | 0.3191 | 0.0156 | 0.0629 |
| $\mathcal{C}_{ab}$ | -0.3043 | -1.5801 | -0.4265 | -0.0209 | -0.0840 |
| $\mathcal{C}_{bb}$ | 0.5022 | 2.6076 | 0.7039 | 0.0345 | 0.1386 |

TABLE XXXII. Coefficients $a_0$, $a_1$, $a_2$, $b_1$, and $b_2$ (in e fm$^3$), Eq. (5), determined for $^{221}$Rn, $^{223}$Rn, $^{223}$Fr, $^{225}$Ra, and $^{229}$Pa from the experimental octupole moments of $^{224}$Ra, $^{226}$Ra, and $^{220}$Rn.

| | $\Delta E$(keV) | From | $a_0$ | $a_1$ | $a_2$ | $b_1$ | $b_2$ |
|---|---|---|---|---|---|---|---|
| | | $^{224}$Ra | −0.38(11) | −0.73(29) | 0.26(11) | −0.019(6) | −0.011(5) |
| $^{221}$Rn | 100$^\dagger$ | $^{226}$Ra | −0.19(09) | −1.27(31) | 0.48(13) | −0.016(4) | −0.009(4) |
| | | $^{220}$Rn | −0.04(10) | −1.69(28) | 0.67(10) | −0.014(5) | −0.007(4) |
| | | $^{224}$Ra | −0.41(10) | −1.34(41) | 0.49(10) | −0.033(10) | −0.015(9) |
| $^{223}$Rn | 100$^\dagger$ | $^{226}$Ra | −0.23(08) | −1.94(38) | 0.70(12) | −0.032(08) | −0.012(7) |
| | | $^{220}$Rn | −0.07(08) | −2.39(41) | 0.86(11) | −0.030(09) | −0.008(8) |
| | | $^{224}$Ra | 0.16(23) | −1.19(72) | 0.31(29) | 0.011(4) | −0.009(7) |
| $^{223}$Fr | 134.48 [12]$^*$ | $^{226}$Ra | −0.03(16) | −0.49(58) | −0.22(28) | 0.024(4) | −0.021(7) |
| | | $^{220}$Rn | −0.20(21) | 0.16(61) | −0.68(25) | 0.033(5) | −0.032(6) |
| | | $^{224}$Ra | −0.22(31) | −3.13(1.48) | 1.96(72) | −0.036(14) | 0.019(23) |
| $^{225}$Ra | 55 [13] | $^{226}$Ra | 0.71(37) | −7.85(1.79) | 4.54(89) | 0.008(17) | 0.038(20) |
| | | $^{220}$Rn | 1.45(34) | −11.50(1.69) | 6.49(93) | 0.042(17) | 0.056(20) |
| | | $^{224}$Ra | −1.04(27) | 0.30(68) | 0.05(35) | 0.030(6) | 0.040(16) |
| $^{229}$Pa | 100$^\dagger$ | $^{226}$Ra | −1.36(20) | 1.52(58) | −0.68(33) | 0.042(5) | 0.022(14) |
| | | $^{220}$Rn | −1.60(26) | 2.52(63) | −1.27(33) | 0.051(7) | 0.007(14) |

$^\dagger$arbitrary value used.

$^*$the second excited $3/2^+$ state is at 160.43 keV.

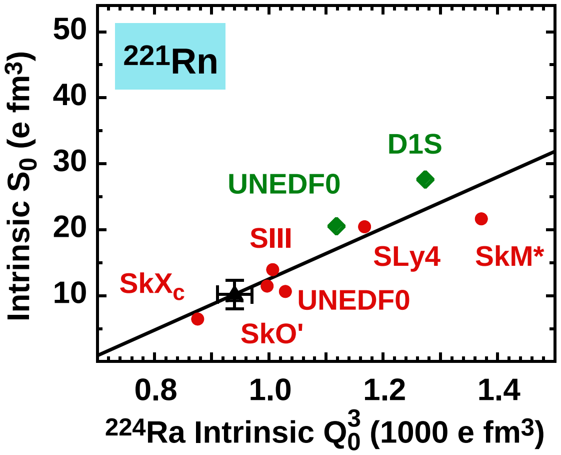


FIG. 5. Intrinsic Schiff moments in $^{221}$Rn correlated with the intrinsic octupole moments in $^{224}$Ra.

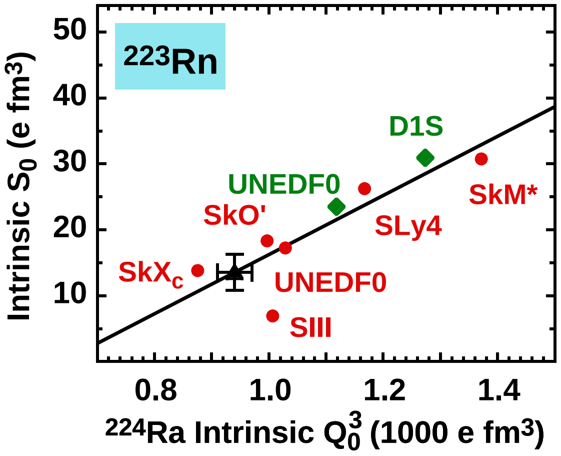


FIG. 6. Intrinsic Schiff moments in $^{223}$Rn correlated with the intrinsic octupole moments in $^{224}$Ra.

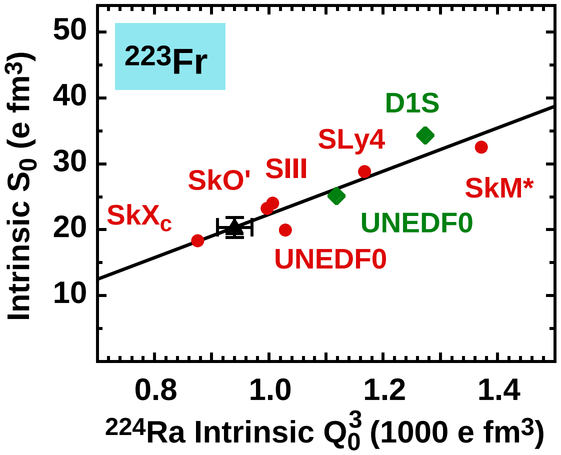


FIG. 7. Intrinsic Schiff moments in $^{223}$Fr correlated with the intrinsic octupole moments in $^{224}$Ra.

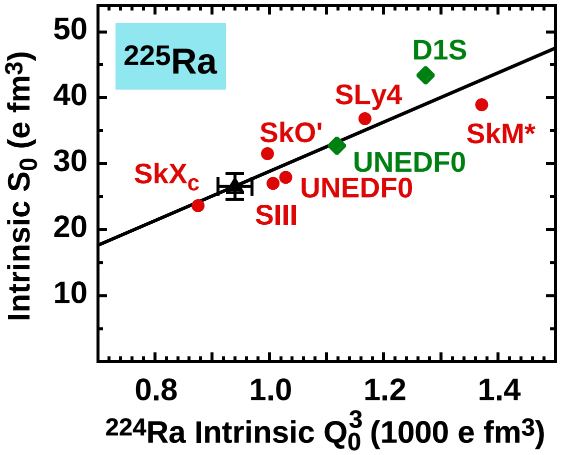


FIG. 8. Intrinsic Schiff moments in $^{225}$Ra correlated with the intrinsic octupole moments in $^{224}$Ra.

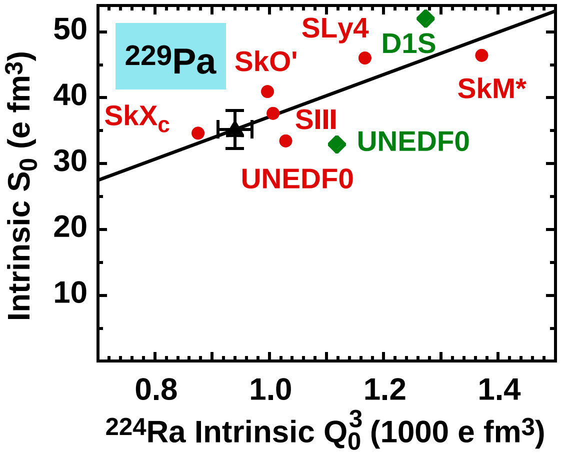


FIG. 9. Intrinsic Schiff moments in $^{229}$Pa correlated with the intrinsic octupole moments in $^{224}$Ra.

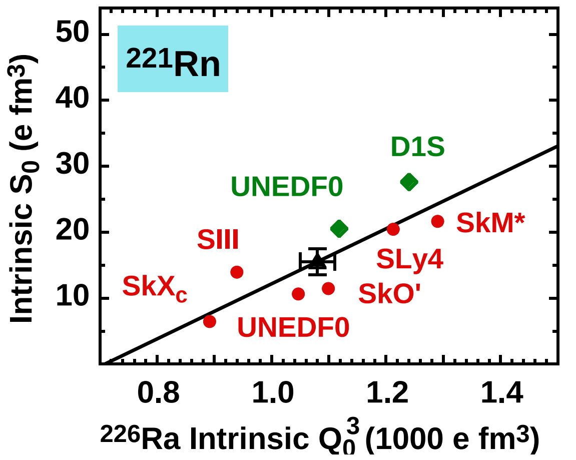


FIG. 10. Intrinsic Schiff moments in $^{221}$Rn correlated with the intrinsic octupole moments in $^{226}$Ra.

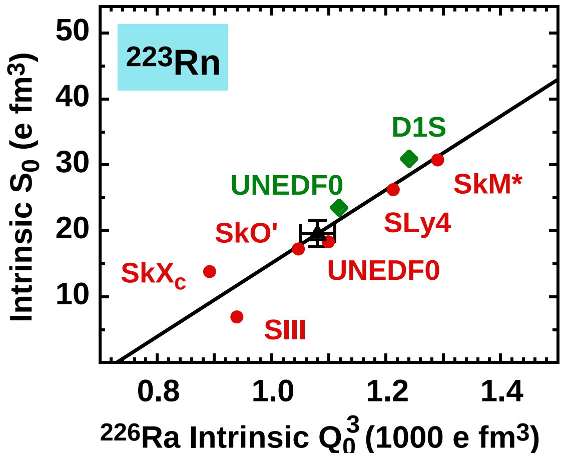


FIG. 11. Intrinsic Schiff moments in $^{223}$Rn correlated with the intrinsic octupole moments in $^{226}$Ra.

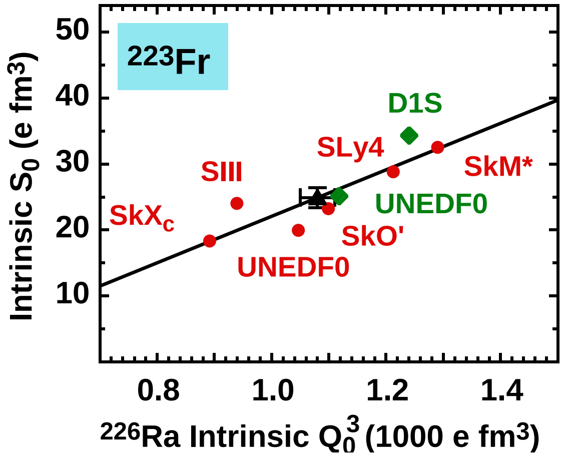


FIG. 12. Intrinsic Schiff moments in $^{223}$Fr correlated with the intrinsic octupole moments in $^{226}$Ra.

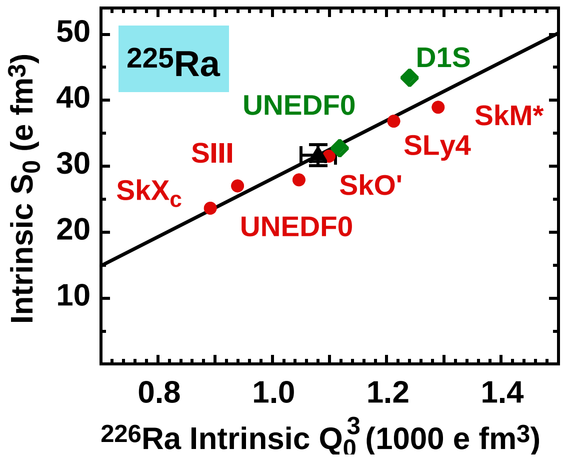


FIG. 13. Intrinsic Schiff moments in $^{225}$Ra correlated with the intrinsic octupole moments in $^{226}$Ra.

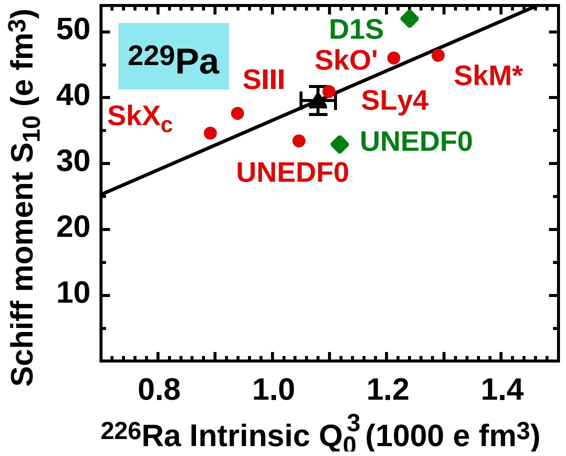


FIG. 14. Intrinsic Schiff moments in $^{229}$Pa correlated with the intrinsic octupole moments in $^{226}$Ra.

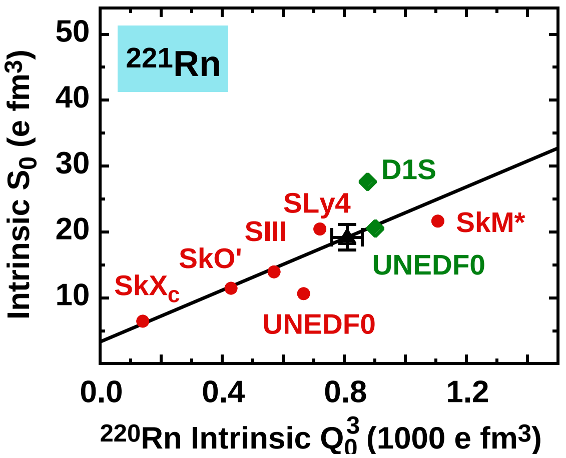


FIG. 15. Intrinsic Schiff moments in $^{221}$Rn correlated with the intrinsic octupole moments in $^{220}$Rn.

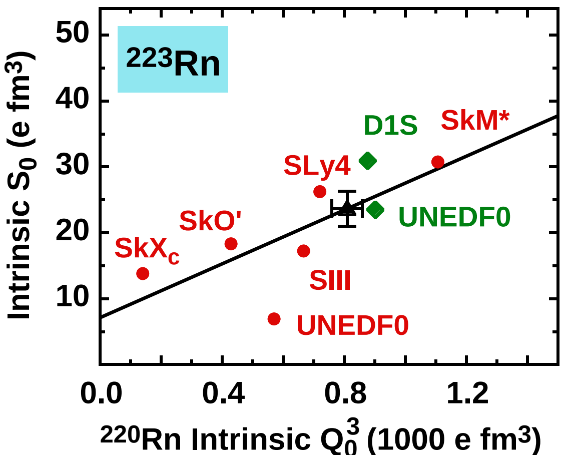


FIG. 16. Intrinsic Schiff moments in $^{223}$Rn correlated with the intrinsic octupole moments in $^{220}$Rn.

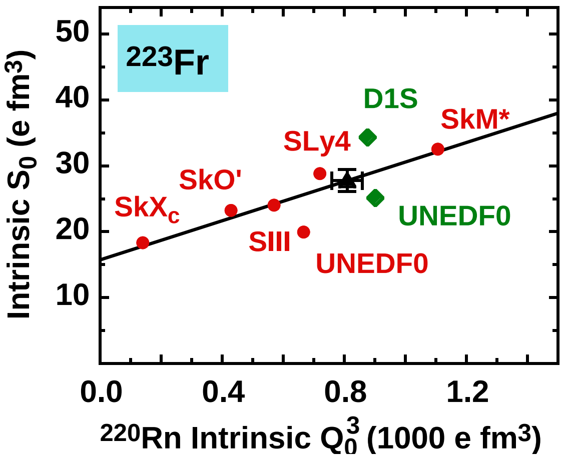


FIG. 17. Intrinsic Schiff moments in $^{223}$Fr correlated with the intrinsic octupole moments in $^{220}$Rn.

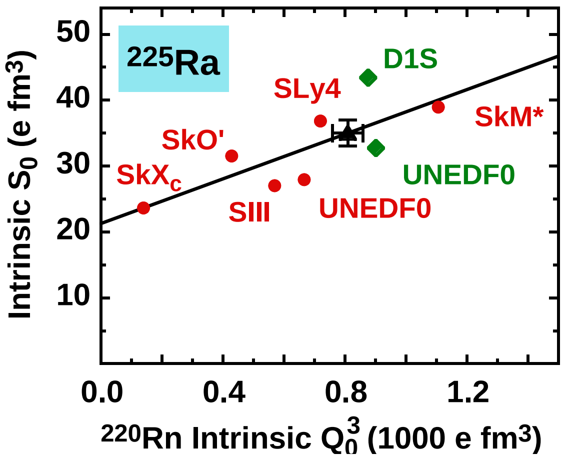


FIG. 18. Intrinsic Schiff moments in $^{225}$Ra correlated with the intrinsic octupole moments in $^{220}$Rn.

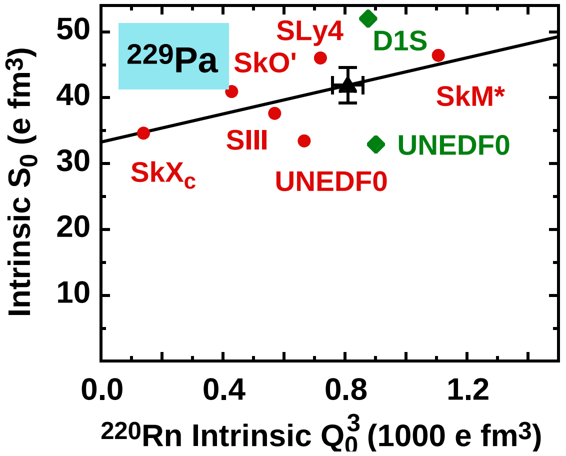


FIG. 19. Intrinsic Schiff moments in $^{229}$Pa correlated with the intrinsic octupole moments in $^{220}$Rn.

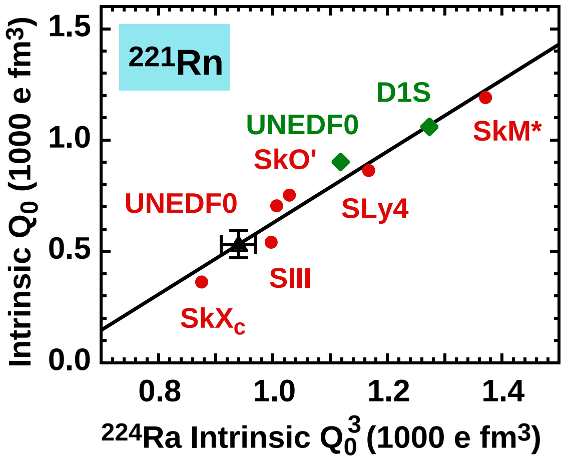


FIG. 20. Intrinsic octupole moments in $^{221}$Rn correlated with the intrinsic octupole moments in $^{224}$Ra.

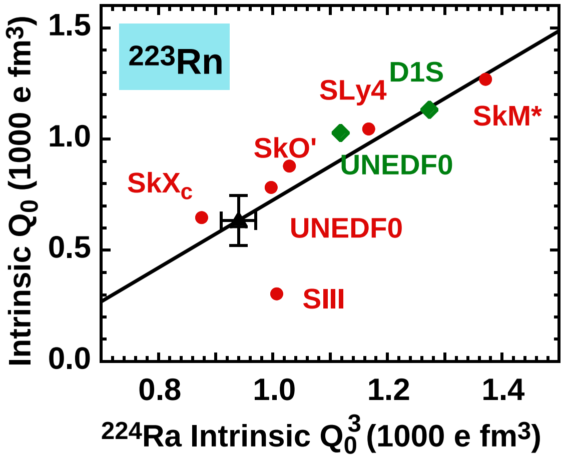


FIG. 21. Intrinsic octupole moments in $^{223}$Rn correlated with the intrinsic octupole moments in $^{224}$Ra.

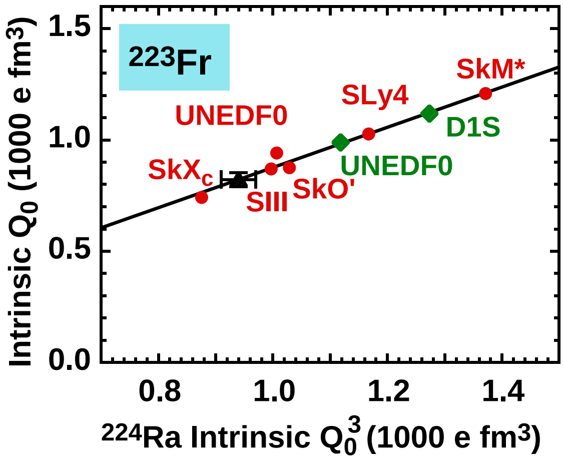


FIG. 22. Intrinsic octupole moments in $^{223}$Fr correlated with the intrinsic octupole moments in $^{224}$Ra.

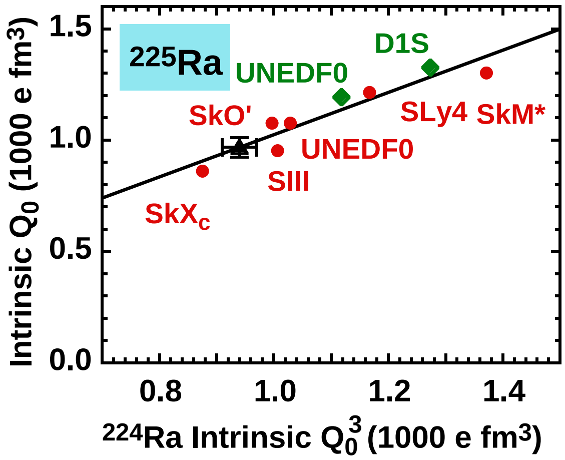


FIG. 23. Intrinsic octupole moments in $^{225}$Ra correlated with the intrinsic octupole moments in $^{224}$Ra.

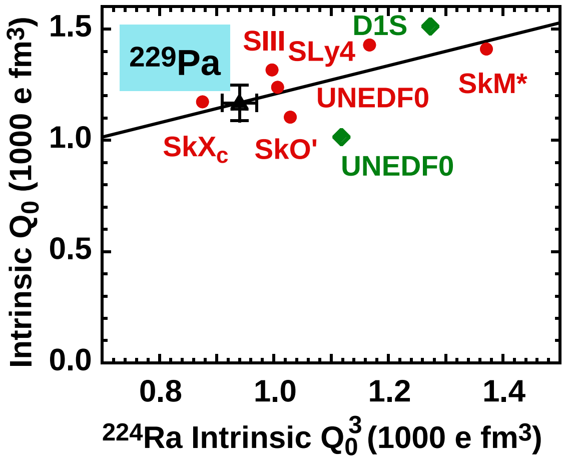


FIG. 24. Intrinsic octupole moments in $^{229}$Pa correlated with the intrinsic octupole moments in $^{224}$Ra.

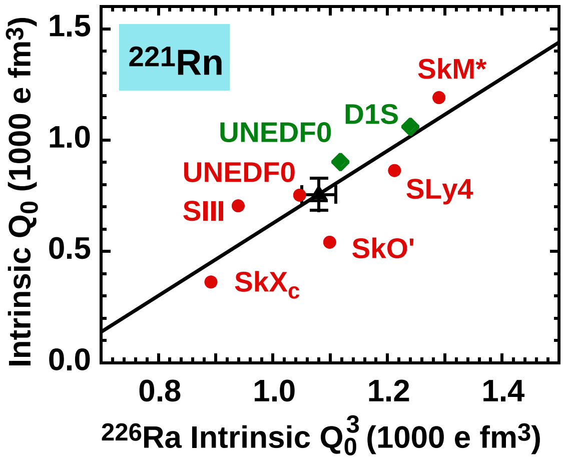


FIG. 25. Intrinsic octupole moments in $^{221}$Rn correlated with the intrinsic octupole moments in $^{226}$Ra.

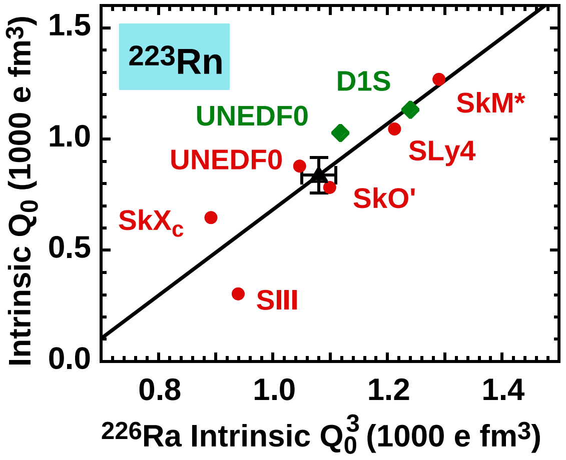


FIG. 26. Intrinsic octupole moments in $^{223}$Rn correlated with the intrinsic octupole moments in $^{226}$Ra.

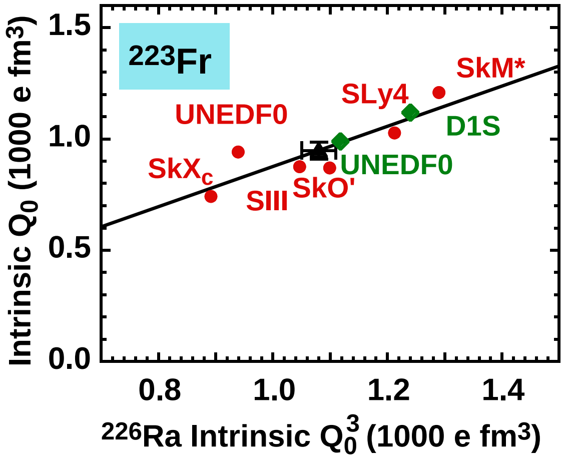


FIG. 27. Intrinsic octupole moments in $^{223}$Fr correlated with the intrinsic octupole moments in $^{226}$Ra.

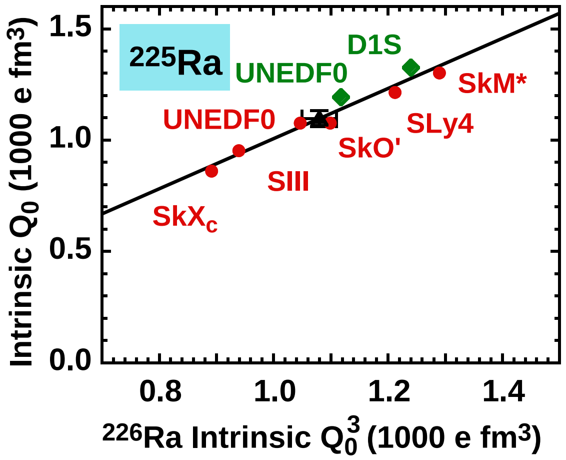


FIG. 28. Intrinsic octupole moments in $^{225}$Ra correlated with the intrinsic octupole moments in $^{226}$Ra.

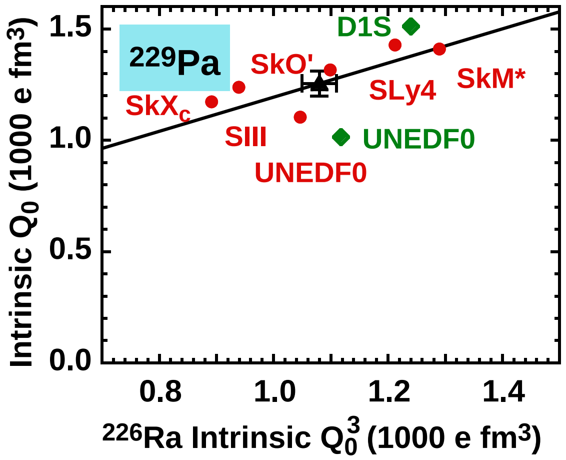


FIG. 29. Intrinsic octupole moments in $^{229}$Pa correlated with the intrinsic octupole moments in $^{226}$Ra.

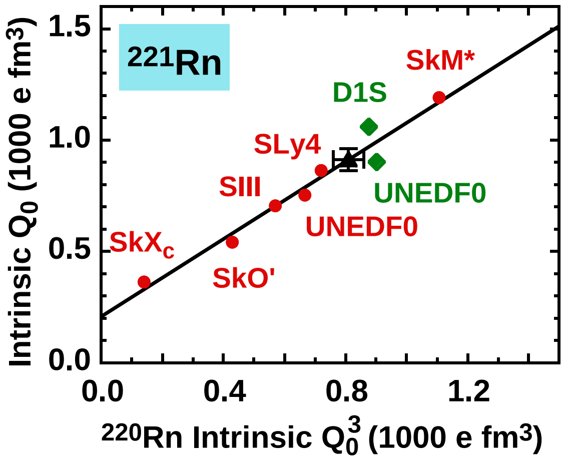


FIG. 30. Intrinsic octupole moments in $^{221}$Rn correlated with the intrinsic octupole moments in $^{220}$Rn.

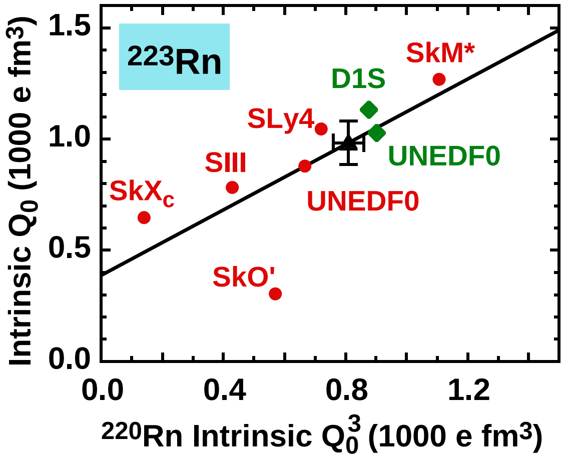


FIG. 31. Intrinsic octupole moments in $^{223}$Rn correlated with the intrinsic octupole moments in $^{220}$Rn.

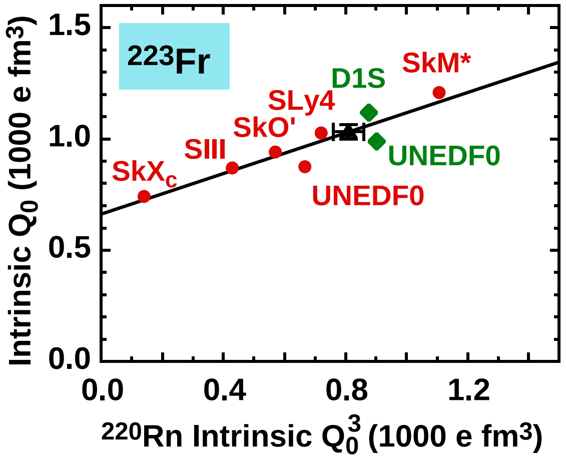


FIG. 32. Intrinsic octupole moments in $^{223}$Fr correlated with the intrinsic octupole moments in $^{220}$Rn.

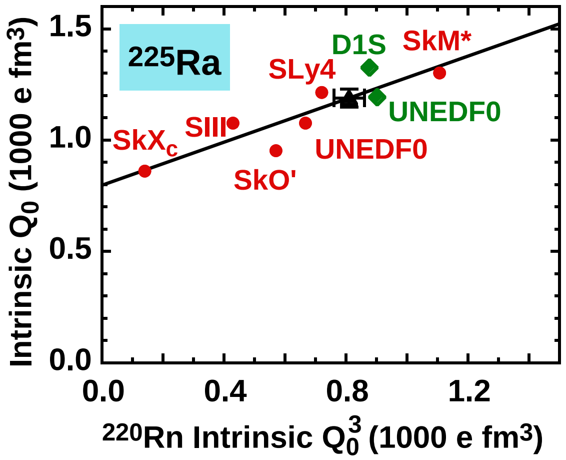


FIG. 33. Intrinsic octupole moments in $^{225}$Ra correlated with the intrinsic octupole moments in $^{220}$Rn.

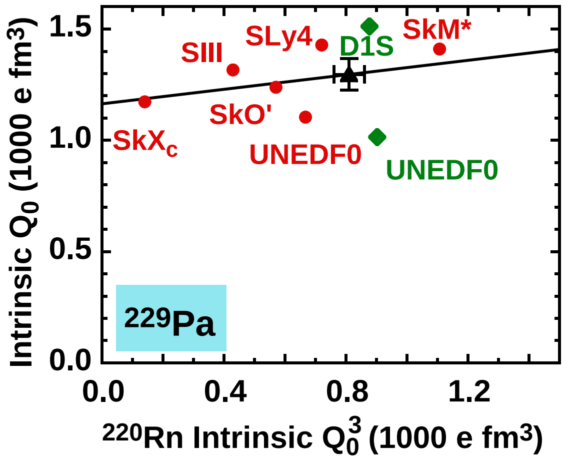


FIG. 34. Intrinsic octupole moments in $^{229}$Pa correlated with the intrinsic octupole moments in $^{220}$Rn.

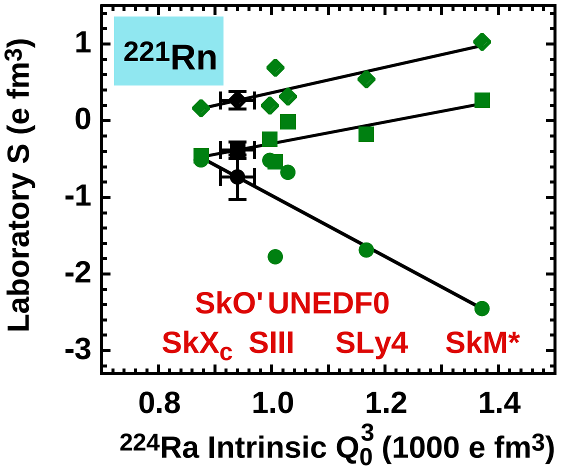


FIG. 35. Coefficients $a_0$ (squares), $a_1$ (circles), and $a_2$ (diamonds), Eq. (5), corresponding to the finite-range terms of $\hat{V}_{PT}$, Eq. (4), determined in $^{221}$Rn for six Skyrme functionals and correlated with the octupole moments in $^{224}$Ra.

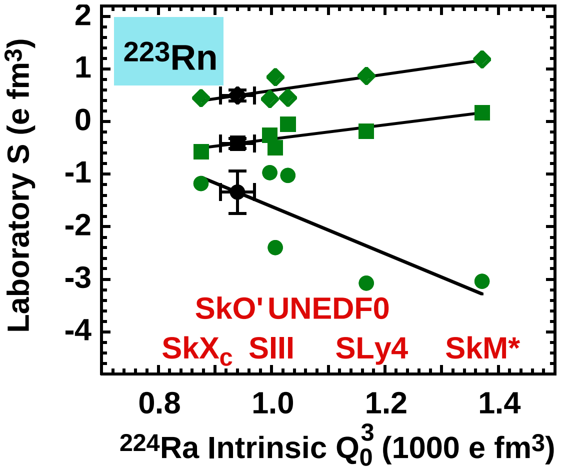


FIG. 36. Same as in Fig. 35, but for $^{223}$Rn correlated with the octupole moments in $^{224}$Ra.

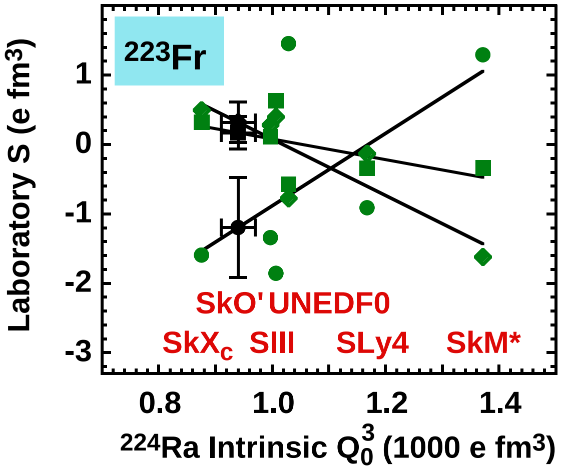


FIG. 37. Same as in Fig. 35, but for $^{223}$Fr correlated with the octupole moments in $^{224}$Ra.

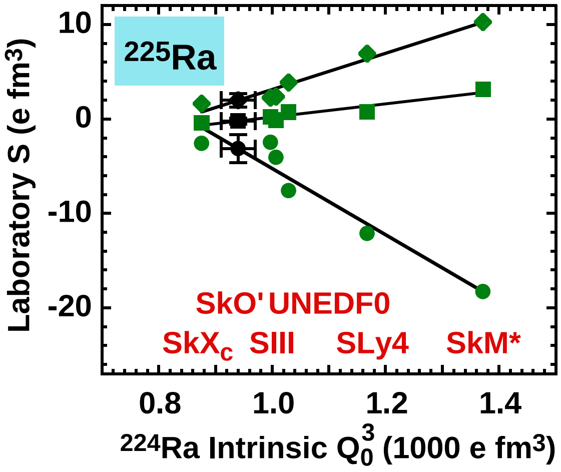


FIG. 38. Same as in Fig. 35, but for $^{225}$Ra correlated with the octupole moments in $^{224}$Ra.

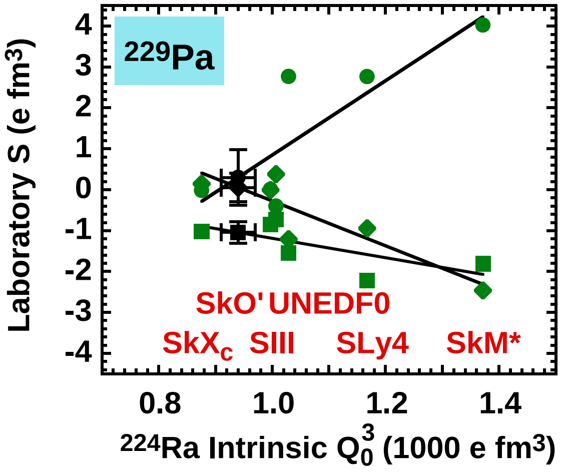


FIG. 39. Same as in Fig. 35, but for $^{229}$Pa correlated with the octupole moments in $^{224}$Ra.

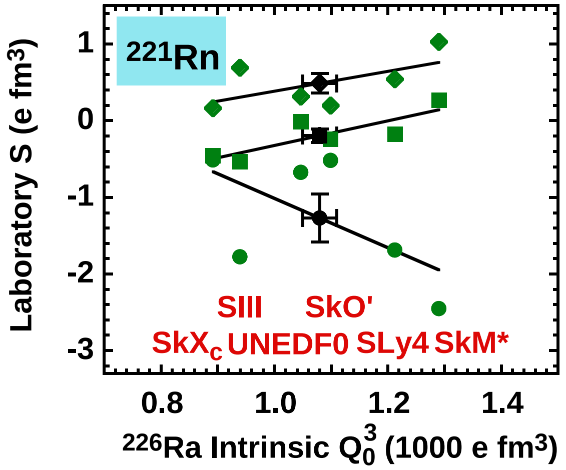


FIG. 40. Same as in Fig. 35, but for $^{221}$Rn correlated with the octupole moments in $^{226}$Ra.

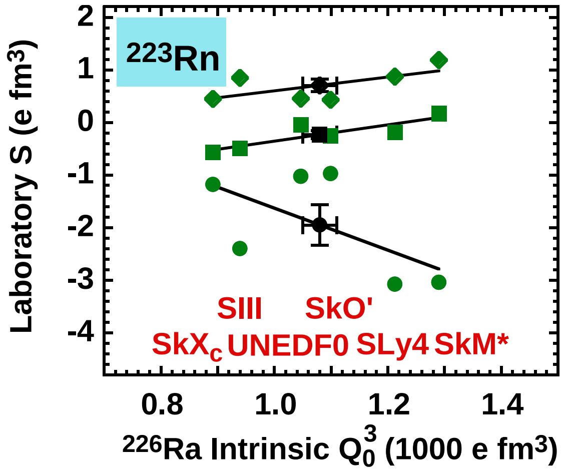


FIG. 41. Same as in Fig. 35, but for $^{223}$Rn correlated with the octupole moments in $^{226}$Ra.

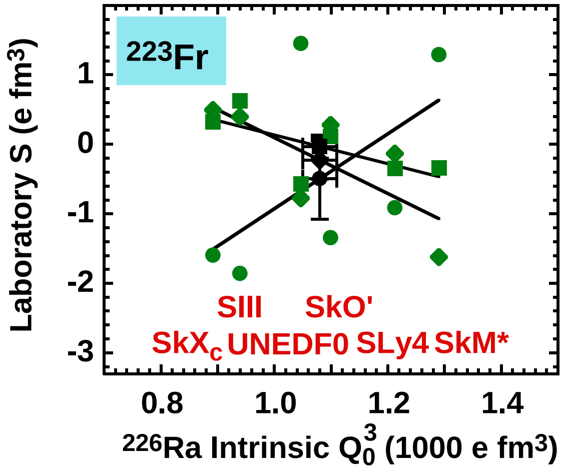


FIG. 42. Same as in Fig. 35, but for $^{223}$Fr correlated with the octupole moments in $^{226}$Ra.

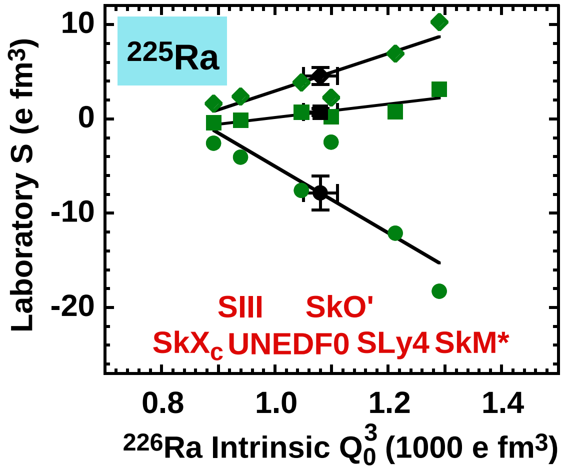


FIG. 43. Same as in Fig. 35, but for $^{225}$Ra correlated with the octupole moments in $^{226}$Ra.

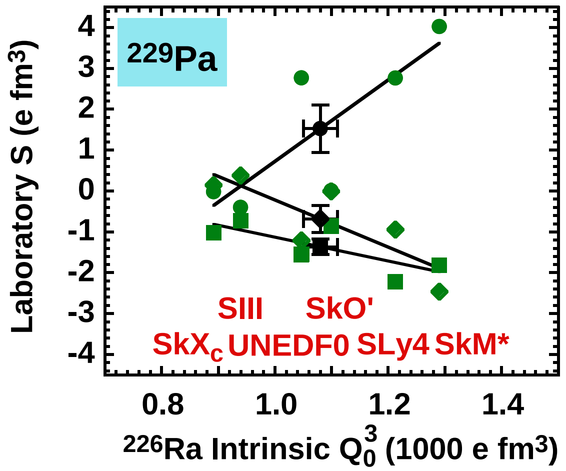


FIG. 44. Same as in Fig. 35, but for $^{229}$Pa correlated with the octupole moments in $^{226}$Ra.

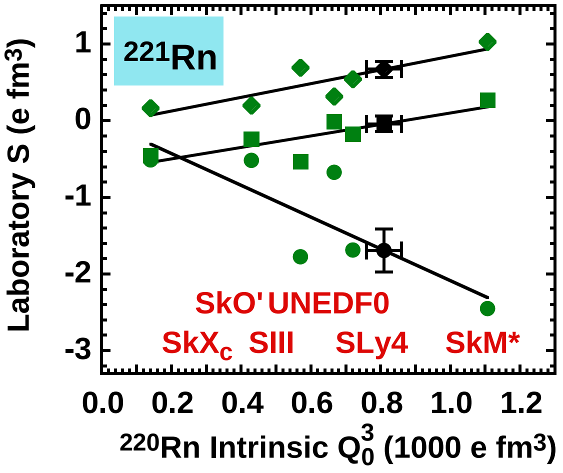


FIG. 45. Same as in Fig. 35, but for $^{221}$Rn correlated with the octupole moments in $^{220}$Rn.

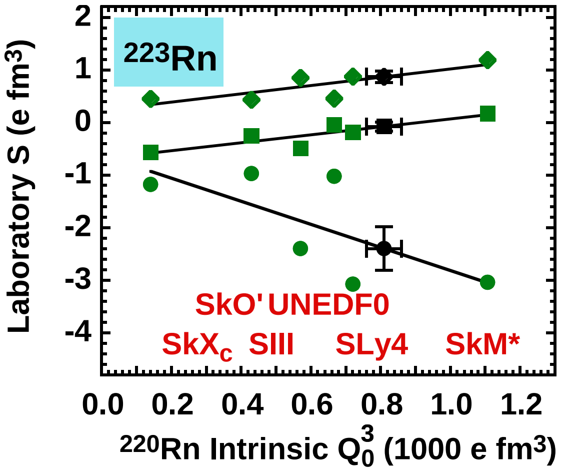


FIG. 46. Same as in Fig. 35, but for $^{223}$Rn correlated with the octupole moments in $^{220}$Rn.

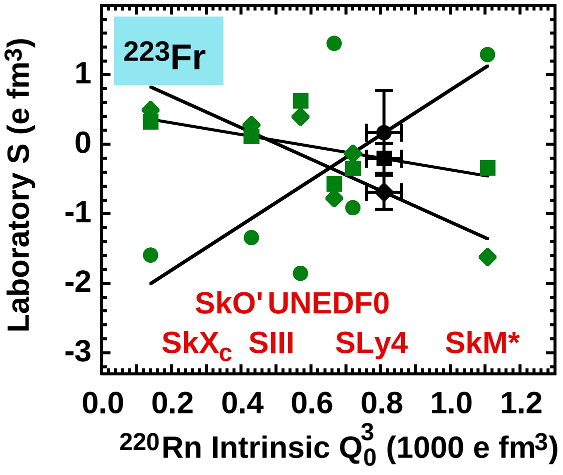


FIG. 47. Same as in Fig. 35, but for $^{223}$Fr correlated with the octupole moments in $^{220}$Rn.

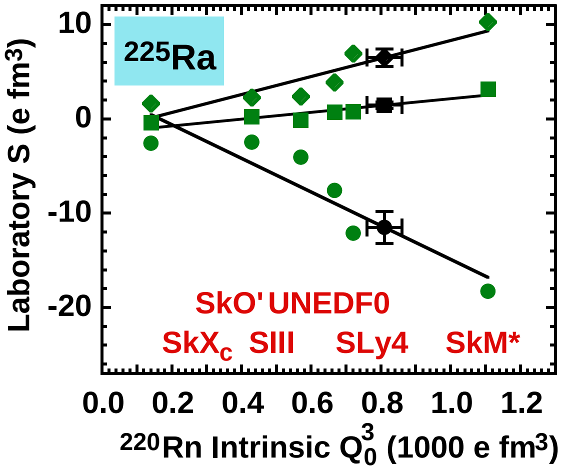


FIG. 48. Same as in Fig. 35, but for $^{225}$Ra correlated with the octupole moments in $^{220}$Rn.

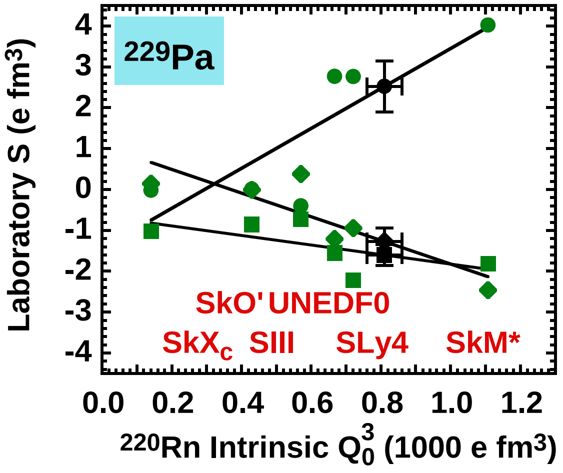


FIG. 49. Same as in Fig. 35, but for $^{229}$Pa correlated with the octupole moments in $^{220}$Rn.

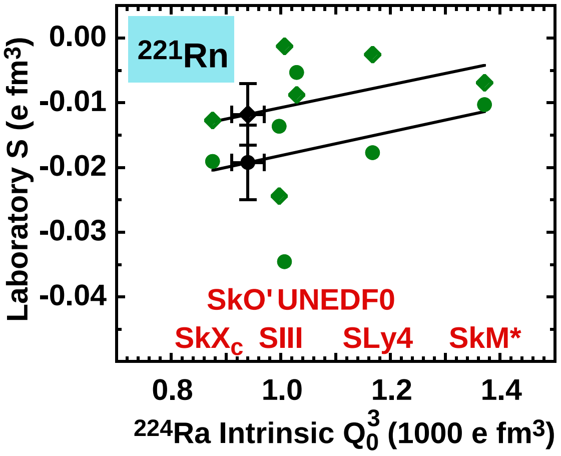


FIG. 50. Coefficients $b_1$ (circles) and $b_2$ (diamonds), Eq. (5), corresponding to the zero-range terms of $\hat{V}_{PT}$, Eq. (4), determined in $^{221}$Rn for six Skyrme functionals and correlated with the octupole moments in $^{224}$Ra.

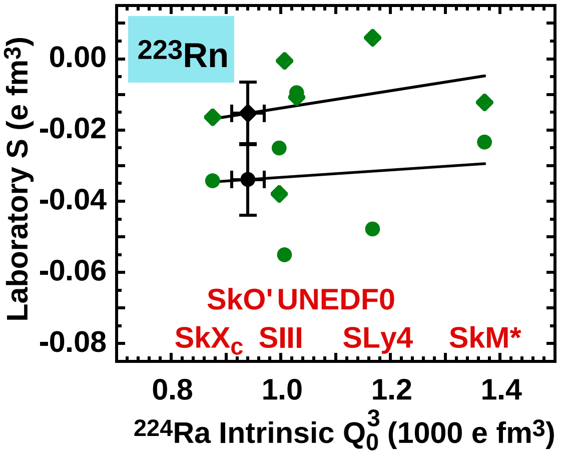


FIG. 51. Same as in Fig. 50, but for $^{223}$Rn correlated with the octupole moments in $^{224}$Ra.

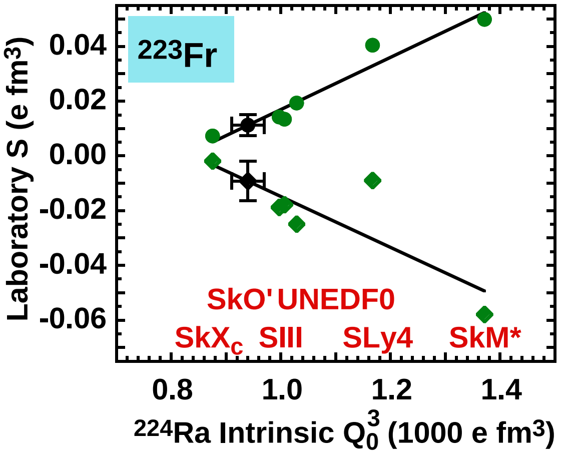


FIG. 52. Same as in Fig. 50, but for $^{223}$Fr correlated with the octupole moments in $^{224}$Ra.

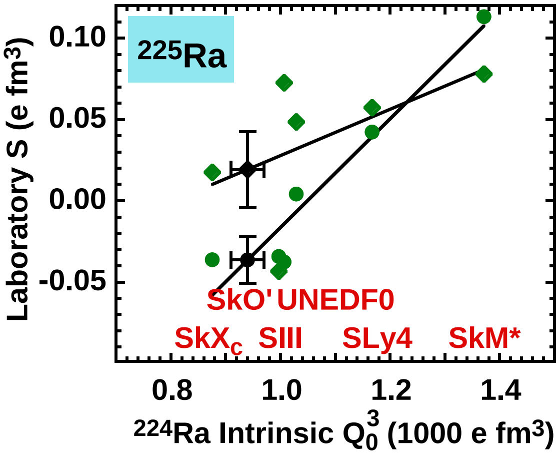


FIG. 53. Same as in Fig. 50, but for $^{225}$Ra correlated with the octupole moments in $^{224}$Ra.

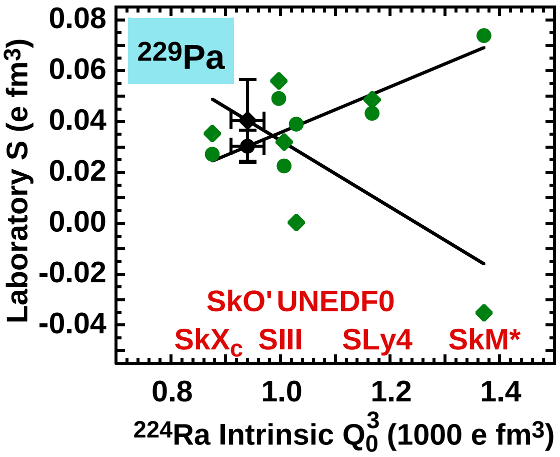


FIG. 54. Same as in Fig. 50, but for $^{229}$Pa correlated with the octupole moments in $^{224}$Ra.

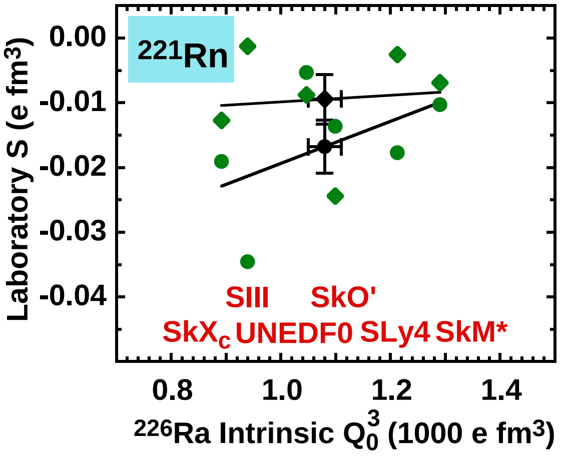


FIG. 55. Same as in Fig. 50, but for $^{221}$Rn correlated with the octupole moments in $^{226}$Ra.

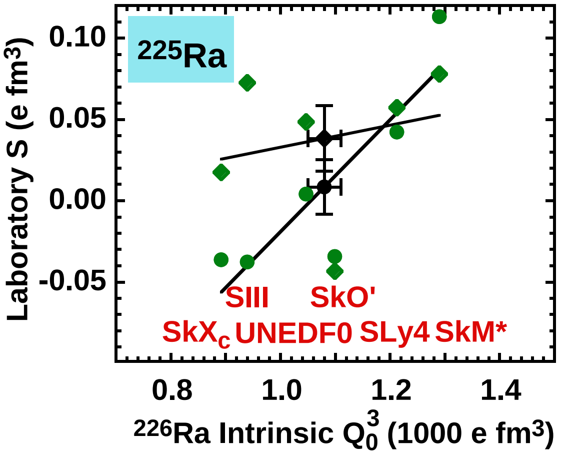


FIG. 58. Same as in Fig. 50, but for $^{225}$Ra correlated with the octupole moments in $^{226}$Ra.

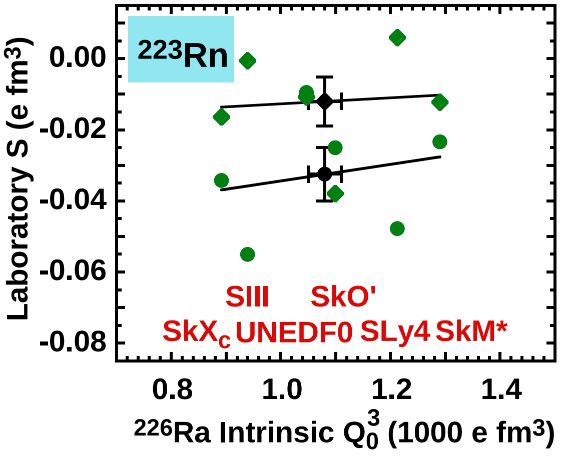


FIG. 56. Same as in Fig. 50, but for $^{223}$Rn correlated with the octupole moments in $^{226}$Ra.

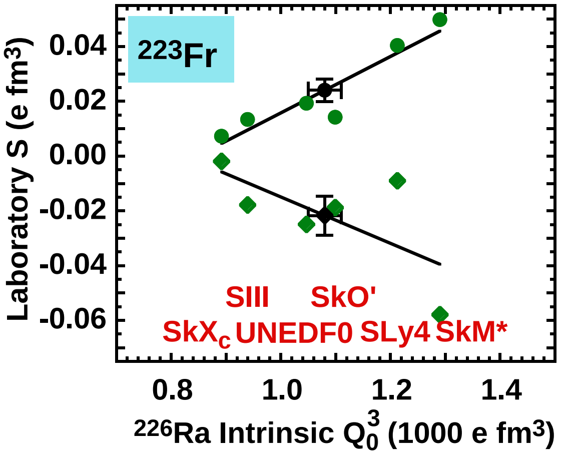


FIG. 57. Same as in Fig. 50, but for $^{223}$Fr correlated with the octupole moments in $^{226}$Ra.

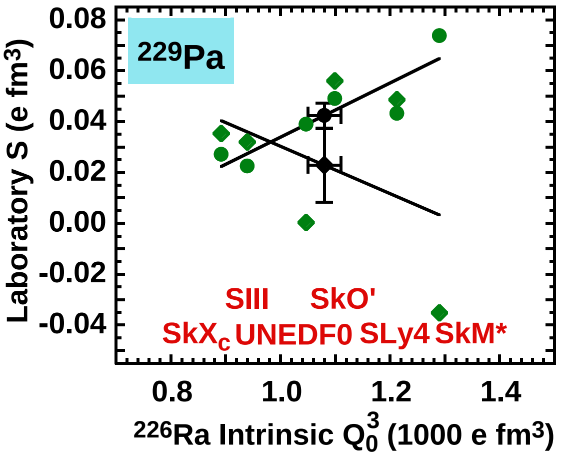


FIG. 59. Same as in Fig. 50, but for $^{229}$Pa correlated with the octupole moments in $^{226}$Ra.

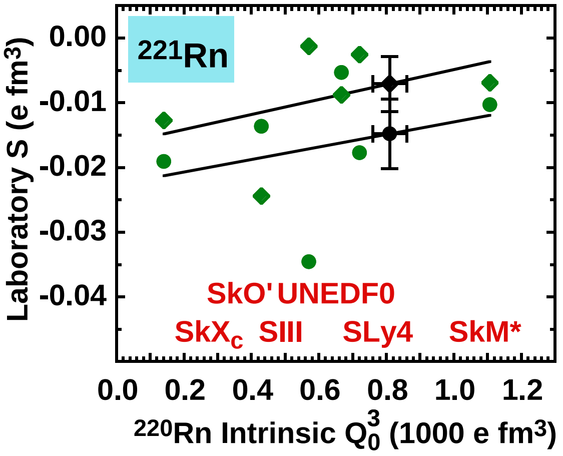


FIG. 60. Same as in Fig. 50, but for $^{221}$Rn correlated with the octupole moments in $^{220}$Rn.

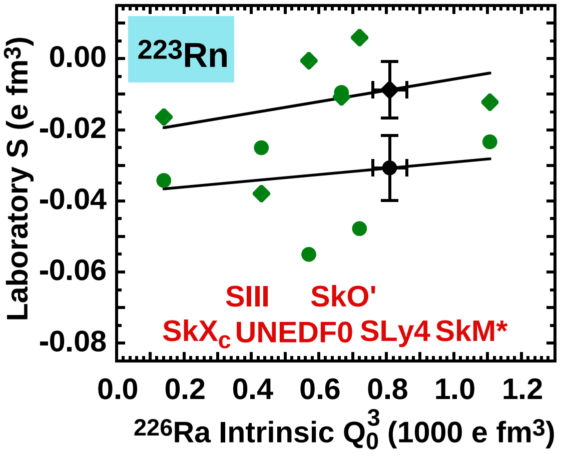


FIG. 61. Same as in Fig. 50, but for $^{223}$Rn correlated with the octupole moments in $^{220}$Rn.

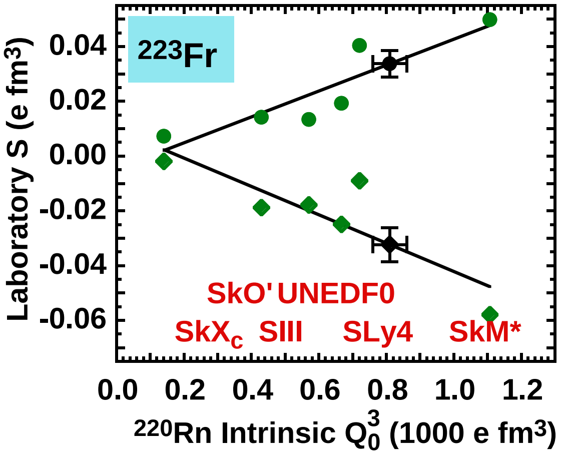


FIG. 62. Same as in Fig. 50, but for $^{223}$Fr correlated with the octupole moments in $^{220}$Rn.

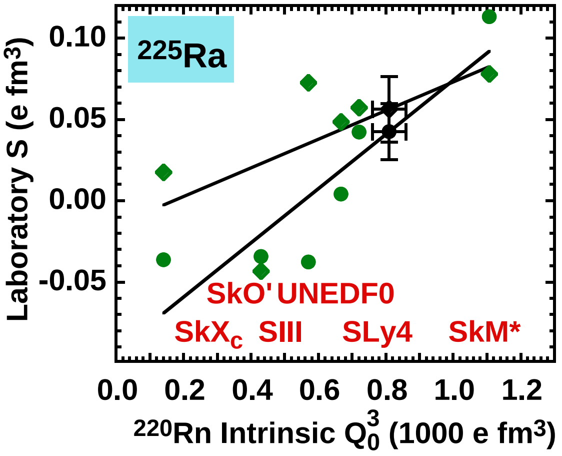


FIG. 63. Same as in Fig. 50, but for $^{225}$Ra correlated with the octupole moments in $^{220}$Rn.

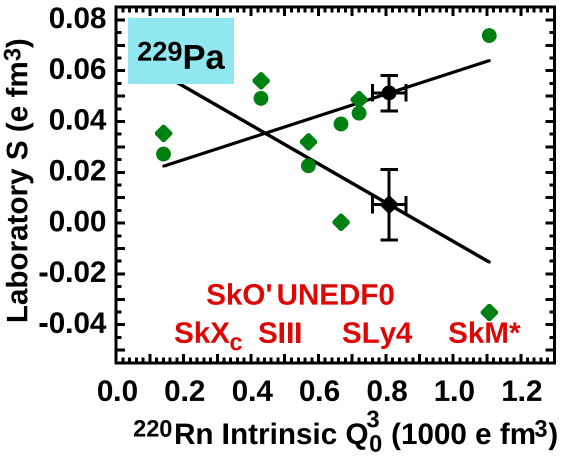


FIG. 64. Same as in Fig. 50, but for $^{229}$Pa correlated with the octupole moments in $^{220}$Rn.

[1] J. Dobaczewski, W. Nazarewicz, and P.-G. Reinhard, Journal of Physics G: Nuclear and Particle Physics **41**, 074001 (2014).
[2] M. Beiner, H. Flocard, N. V. Giai, and P. Quentin, Nuclear Physics A **238**, 29 (1975).
[3] J. Bartel, P. Quentin, M. Brack, C. Guet, and H.-B. Håkansson, Nuclear Physics A **386**, 79 (1982).
[4] P.-G. Reinhard, Nucl. Phys. A **649**, 305c (1999).
[5] B. A. Brown, Phys. Rev. C **58**, 220 (1998).
[6] E. Chabanat, P. Bonche, P. Haensel, J. Meyer, and R. Schaeffer, Nuclear Physics A **635**, 231 (1998).
[7] M. Kortelainen, T. Lesinski, J. Moré, W. Nazarewicz, J. Sarich, N. Schunck, M. V. Stoitsov, and S. Wild, Phys. Rev. C **82**, 024313 (2010).
[8] J. Berger, M. Girod, and D. Gogny, Computer Physics Communications **63**, 365 (1991).
[9] R. T. Birge, Phys. Rev. **40**, 207 (1932).
[10] L. P. Gaffney, P. A. Butler, M. Scheck, A. B. Hayes, F. Wenander, M. Albers, B. Bastin, C. Bauer, A. Blazhev, S. Bönig, N. Bree, J. Cederkäll, T. Chupp, D. Cline, T. E. Cocolios, T. Davinson, H. De Witte, J. Diriken, T. Grahn, A. Herzan, M. Huyse, D. G. Jenkins, D. T. Joss, N. Kesteloot, J. Konki, M. Kowalczyk, T. Kröll, E. Kwan, R. Lutter, K. Moschner, P. Napiorkowski, J. Pakarinen, M. Pfeiffer, D. Radeck, P. Reiter, K. Reynders, S. V. Rigby, L. M. Robledo, M. Rudigier, S. Sambi, M. Seidlitz, B. Siebeck, T. Stora, P. Thoele, P. Van Duppen, M. J. Vermeulen, M. von Schmid, D. Voulot, N. Warr, K. Wimmer, K. Wrzosek-Lipska, C. Y. Wu, and M. Zielinska, Nature **497**, 199 (2013).
[11] H. Wollersheim, H. Emling, H. Grein, R. Kulessa, R. Simon, C. Fleischmann, J. de Boer, E. Hauber, C. Lauterbach, C. Schandera, P. Butler, and T. Czosnyka, Nuclear Physics A **556**, 261 (1993).
[12] R. K. Sheline, C. F. Liang, P. Paris, J. Kvasil, and D. Nosek, Phys. Rev. C **51**, 1708 (1995).
[13] R. Helmer, M. Lee, C. Reich, and I. Ahmad, Nuclear Physics A **474**, 77 (1987).
